# Supplementary material for: Correct-by-Design Teamwork Plans for Multi-Agent Systems
Source: arXiv:2301.01257 source file (2023-05-12)
Supplement: Supplementary file 1 [file appendix.tex]

% !TEX root = ../aamas23.tex
\section{Appendix}\label{appendix}

\begin{proof}[Proof of Theorem 5.5]
It is sufficient to prove that for every composite parameter state $\epsilon$, the following relation:
\[\mathcal{R}_{\epsilon\backslash p}=\set{((s_1,p),(s_2,p))~|~\mbox{for all states}\ s_1,s_2,\ s.t.\ (s_1\sim_{\epsilon}s_2)}\] is a $(\epsilon\backslash p)$-bisimulation.

Recall that $\|$ is a commutative monoid, and thus it is closed under commutativity, associativity, and $\mathsf{Id}$-element. Thus, the rest of the proof is by induction on the length $(w)$ of the projection with respect to the history of the parameter TS. The key idea of the proof is that send actions of the form $(c,!,\upsilon)$ can only originate from within the composition, i.e., can be sent by $s_1$ (or $s_2$) or $\epsilon$. Moreover, a receive action of the form $(c,?,\upsilon)$ can only happen jointly with a corresponding send while the latter is autonomous.

\begin{itemize}[label={$\bullet$}, topsep=2pt, itemsep=2pt, leftmargin=10pt]
\item Consider $w=0$: then \[\mathcal{R}_{\epsilon}=\set{((s_1,0),(s_2,0))~|~\mbox{for all states}\ s_1,s_2,\ s.t.\ (s_1\sim_{\epsilon}s_2)}\] where $0$ is a sink state as defined before. This is a $(\epsilon)$-bisimulation by definition.

\item Assume it holds for $w=n-1$: then we need to prove it for $w+1$, i.e., $w=n$. This means that we are projecting the whole composite state and we need to prove that: 
 \[\mathcal{R}_{0}=\set{((s_1,\epsilon),(s_2,\epsilon))~|~\mbox{for all states}\ s_1,s_2,\ s.t.\ (s_1\sim_{\epsilon}s_2)}\]  is a $(0)$-bisimulation.
 
 Since the parameter is empty then all message-sends can only originate from the composition $(s,\epsilon)$. The empty parameter cannot influence the composition. Now, we need to check if the items of Def.~\ref{def:bisim} (and their symmetric cases) hold. We do that one by one.
 
 Consider the case: $((s_1,\epsilon),{(c,!,\upsilon)},(s'_1,\epsilon'))\in\Delta$. By $\Delta$ of the team composition in Def.~\ref{def:comp}, we have that this transition can be derived because of the following cases:
 \begin{itemize}[label={$\bullet$}, topsep=2pt, itemsep=2pt, leftmargin=10pt]
 \item $(s_1,{(c,!,\upsilon)},s'_1)\in\Delta_1$, $c\in\listen(\epsilon)$, and $(\epsilon,{(c,?,\upsilon)},\epsilon')\in\Delta_{\mathcal{E}}$. This means that $s_1\rTo{(c,!,\upsilon)!}s'_1$ and $(s_1,\epsilon)\rTo{(c,!,\upsilon)!}(s'_1,\epsilon')$. But $s_1\sim_{\epsilon}s_2$, and thus  $s_2\rTo{(c,!,\upsilon)!}s'_2$ and $(s'_1,s'_2)\in\mathcal{R}_{\epsilon'}$.
 
 By Def.~\ref{def:comp}, we have also that $((s_2,\epsilon),{(c,!,\upsilon)},(s'_2,\epsilon'))\in\Delta$, 
 
 and thus $(s_2,\epsilon)\rTo{(c,!,\upsilon)!}(s'_2,\epsilon')$. Clearly, $((s'_1,\epsilon'),(s'_2,\epsilon'))\in\mathcal{R}_{0}$ as required.
 
 \item The symmetric case when $(s_2,{(c,!,\upsilon)},s'_2)\in\Delta_1$, $c\in\listen(\epsilon)$, and $(\epsilon,{(c,?,\upsilon)},\epsilon')\in\Delta_{\mathcal{E}}$. It holds in the same way.
 
 \item $(s_1,{(c,!,\upsilon)},s'_1)\in\Delta_1$, $c\not\in\listen(\epsilon)$, and $\epsilon={\epsilon'}$. This means that $s_1\rTo{(c,!,\upsilon)!}s'_1$ and $(s_1,\epsilon)\rTo{(c,!,\upsilon)!}(s'_1,\epsilon)$. But $s_1\sim_{\epsilon}s_2$, and thus  $s_2\rTo{(c,!,\upsilon)!}s'_2$ and $(s'_1,s'_2)\in\mathcal{R}_{\epsilon}$.
 
 By Def.~\ref{def:comp}, we have also that $((s_2,\epsilon),{(c,!,\upsilon)},(s'_2,\epsilon))\in\Delta$, 
 
 and thus $(s_2,\epsilon)\rTo{(c,!,\upsilon)!}(s'_2,\epsilon)$. Clearly, $((s'_1,\epsilon),(s'_2,\epsilon))\in\mathcal{R}_{0}$ as required.
 
\item The symmetric case when $(s_2,{(c,!,\upsilon)},s'_2)\in\Delta_1$, $c\not\in\listen(\epsilon)$, and $\epsilon={\epsilon'}$. It holds in the same way.

\item  $c\not\in\listen(s_1)$, $(s_1= s'_1)$, and $(\epsilon,{(c,!,\upsilon)},\epsilon')\in\Delta_{\mathcal{E}}$. This holds vacuously.
 
 \item  The symmetric case when $c\not\in\listen(s_2)$, $(s_2= s'_2)$, and $(\epsilon,{(c,!,\upsilon)},\epsilon')\in\Delta_{\mathcal{E}}$ holds vacuously.

The interesting cases are the following:

\item  $c\in\listen(s_1)$, $(s_1,{(c,?,\upsilon)},s'_1)\in\Delta_1$, $L(s_1)= L(s'_1)$, and $(\epsilon,{(c,!,\upsilon)},\epsilon')\in\Delta_{\mathcal{E}}$. This means that $s_1\rTo{\tau_{(c,!,\upsilon)}}s'_1$ and $(s_1,\epsilon)\rTo{{(c,!,\upsilon)!}}(s'_1,\epsilon')$. But $s_1\sim_{\epsilon}s_2$, and thus either \rom{1}: $s_2\rTo{\tau_{(c,!,\upsilon)}}$ and this is direct matching. Note that the latter case handles branching. It does not allow a state to simulate another one by only supplying a sequence of discards, when it has the possibility to branch with exactly the same message-receive to a non-equivalent state. Notice that is captured by the composition in Def.~\ref{def:comp} in combination with {Property~\ref{pr:brd}}. That is, a state that can supply a receive transition (it is also listening by Property~\ref{pr:brd}) cannot avoid but to be involved in the interaction. Indeed, without this case Def.~\ref{def:comp} will allow direction application of receive, and thus prove that the bisimulation is not congruence; 

\rom{2} or  $s_2\not\rTo{\tau_{(c,!,\upsilon)}}$ then $\exists s'_2, \epsilon'',\  \ s_2\
	(\RTO{\tau}{\star})_{\epsilon''}^{\epsilon}\ s'_2$ and $(s'_1,s'_2)\in\mathcal{R}_{\epsilon'}$.
 
 We need to prove that $ s_2\
	(\RTO{\tau}{\star})_{\epsilon''}^{\epsilon}\ s'_2$, given that $(\epsilon''\rTo{a_1!}\dots\rTo{a_m!})^{\star}\epsilon\rTo{(c,!,\upsilon)!}\epsilon'$ for some length $m$ and $((s'_1,\epsilon'),(s'_2,\epsilon'))\break\in\mathcal{R}_{0}$. Recall that $s_2$ cannot do a sequence of discards without being supplied with matching sends from the parameter state. That is why the parameter should have the possibility to supply a matching send for each discard step for $s_2$ otherwise $s_2$ cannot do the simulation from its side.
	
By induction on the length of $(\RTO{\tau}{\star})_{\epsilon''}^{\epsilon}$

Consider the $\size{(\RTO{\tau}{\star})_{\epsilon''}^{\epsilon}}=0$ then this means that $s_2=s'_2$, $\epsilon''=\epsilon$ and $c\not\in\listen(s_2)$ 

 By Def.~\ref{def:comp}, we have  that $((s_2,\epsilon),{(c,!,\upsilon)},(s_2,\epsilon'))\in\Delta$. That is,  
$(s_2,\epsilon)\rTo{{(c,!,\upsilon)!}}(s_2,\epsilon')$ and $((s'_1,\epsilon'),(s_2,\epsilon'))\in\mathcal{R}_{0}$ as required.

Assume it holds for $\size{(\RTO{\tau}{\star})_{\epsilon''}^{\epsilon}}=k$, we need to prove it for $k+1$.
That is, we need to prove that $ (s_2,\epsilon'')\rTo{a_1!}\dots\rTo{a_k!}_k(s''_2,\epsilon)\rTo{(c,!,\upsilon)!}(s'_2,\epsilon')$ for $k$-sends, and $((s'_1,\epsilon'),(s'_2,\epsilon'))\in\mathcal{R}_{0}$.
 By Def.~\ref{def:comp} and the induction hypothesis, we can can reach $(s''_2,\epsilon)$ from which we have $(s''_2,\epsilon)\rTo{(c,!,\upsilon)!}(s'_2,\epsilon')$. This means that $s''_2\rTo{\tau_{(c,!,\upsilon)}}s'_2$, i.e., $(s''_2,{(c,?,\upsilon)},s'_2)\in\Delta_2$ and $c\in\listen(s''_2)$. We apply Def.~\ref{def:comp} and we get that $((s'_1,\epsilon'),(s_2,\epsilon'))\in\mathcal{R}_{0}$ as required.

\item  $c\in\listen(s_1)$, $(s_1,{(c,?,\upsilon)},s'_1)\in\Delta_1$, $L(s_1)\neq L(s'_1)$, and $(\epsilon,{(c,!,\upsilon)},\epsilon')\in\Delta_{\mathcal{E}}$. This means that $s_1\rTo{(c,!,\upsilon)?}s'_1$ and $(s_1,\epsilon)\rTo{(c,!,\upsilon)!}(s'_1,\epsilon')$. But $s_1\sim_{\epsilon}s_2$, and thus either $s_2\rTo{(c,!,\upsilon)?}$ and this is direct matching.

or  $s_2\not\rTo{(c,!,\upsilon)?}$ then $\exists s'_2,s''_2, \epsilon'',\  \ s_2\
	(\RTO{\tau}{\star})_{\epsilon''}^{\epsilon}\ s''_2\rTo{(c,!,\upsilon)?}\ s'_2$ and $(s'_1,s'_2)\in\mathcal{R}_{\epsilon'}$.
 
This case holds by a similar induction on the length of the transition as in the previous case. 
 
 \end{itemize}

\end{itemize}
\end{proof}
